# Supplementary material for: Estimating the Number of HTTP/3 Responses in QUIC Using Deep Learning
Source: arXiv:2410.06140 source file (2025-04-28)
Supplement: Supplementary file 1 [file appendix.tex]

\section{Appendices}

\begin{table*}[ht]
\centering
\caption{$T=0.1$-second window dataset: Images per class value, per server.}
\begin{resizebox}{\textwidth}{!}{%
\begin{tabular}{|c|c|c|c|c|c|c|c|c|c|c|c|c|c|c|c|c|c|}
\hline
Class & youtube.com & semrush.com & discord.com & instagram.com & mercedes-benz.com & bleacherreport.com & nicelocal.com & facebook.com & pcmag.com & logitech.com & google.com & cdnetworks.com & independent.co.uk & cloudflare.com & jetbrains.com \\ \hline
0     & 68,730       & 113,947      & 190,942      & 10,340        & 4,255              & 421,728           & 113,581        & 9,345        & 996,908    & 14,435      & 37,501     & 40,332         & 126,199          & 417,474       & 10,993        \\ \hline
1     & 32,180       & 137,842      & 156,369      & 2,958         & 1,154              & 190,606           & 103,038        & 4,503        & 141,714    & 14,785      & 18,567     & 50,600         & 37,183           & 506,356       & 5,392         \\ \hline
2     & 13,426       & 53,672       & 126,360      & 1,215         & 661               & 39,619            & 119,751        & 2,219        & 29,480     & 9,181       & 7,584      & 39,329         & 6,004            & 192,943       & 4,285         \\ \hline
3     & 7,961        & 32,087       & 63,141       & 621          & 523               & 19,860            & 71,226         & 1,374        & 4,330      & 4,206       & 4,637      & 21,876         & 1,890            & 120,638       & 2,202         \\ \hline
4     & 5,733        & 23,880       & 37,571       & 314          & 449               & 33,013            & 42,885         & 922         & 2,996      & 5,166       & 3,899      & 14,017         & 1,138            & 54,700        & 1,579         \\ \hline
5     & 9,184        & 17,406       & 21,260       & 359          & 442               & 20,144            & 28,455         & 349         & 2,145      & 1,620       & 2,484      & 8,940          & 811             & 33,681        & 1,692         \\ \hline
6     & 1,210        & 10,376       & 8,374        & 472          & 443               & 14,649            & 18,191         & 545         & 2,429      & 1,238       & 1,576      & 6,523          & 1,129            & 16,264        & 1,811         \\ \hline
7     & 751         & 7,981        & 5,235        & 338          & 281               & 9,473             & 16,304         & 4,143        & 1,788      & 719        & 1,572      & 4,522          & 522             & 3,397         & 1,154         \\ \hline
8     & 488         & 7,624        & 3,342        & 171          & 339               & 17,508            & 12,342         & 326         & 813       & 338        & 998       & 3,417          & 383             & 987          & 1,616         \\ \hline
9     & 111         & 7,292        & 2,757        & 140          & 237               & 3,735             & 11,027         & 324         & 339       & 417        & 493       & 2,421          & 290             & 326          & 2,635         \\ \hline
10    & 39          & 8,132        & 2,251        & 66           & 209               & 7,510             & 10,050         & 383         & 213       & 348        & 345       & 2,040          & 240             & 195          & 745          \\ \hline
11    & 14          & 8,308        & 1,143        & 9            & 171               & 2,587             & 5,406          & 275         & 249       & 370        & 297       & 1,847          & 171             & 165          & 764          \\ \hline
12    & 9           & 5,557        & 1,264        & 0            & 145               & 272              & 2,861          & 289         & 84        & 801        & 261       & 1,706          & 163             & 98           & 66           \\ \hline
13    & 11          & 5,109        & 768         & 0            & 129               & 230              & 1,397          & 332         & 148       & 462        & 200       & 1,569          & 123             & 113          & 0            \\ \hline
14    & 7           & 4,211        & 683         & 0            & 151               & 270              & 736           & 136         & 8         & 717        & 218       & 1,289          & 108             & 80           & 0            \\ \hline
15    & 4           & 4,964        & 685         & 0            & 91                & 184              & 342           & 313         & 5         & 464        & 146       & 1,415          & 109             & 96           & 0            \\ \hline
16    & 6           & 6,328        & 318         & 0            & 68                & 201              & 123           & 48          & 41        & 473        & 169       & 1,437          & 68              & 74           & 0            \\ \hline
17    & 8           & 6,029        & 311         & 0            & 83                & 176              & 125           & 55          & 18        & 441        & 99        & 1,229          & 64              & 55           & 0            \\ \hline
18    & 4           & 5,442        & 348         & 0            & 83                & 73               & 87            & 26          & 21        & 221        & 77        & 1,014          & 65              & 41           & 0            \\ \hline
19    & 8           & 4,797        & 271         & 0            & 40                & 47               & 31            & 56          & 8         & 211        & 76        & 998           & 38              & 16           & 0            \\ \hline
20    & 5           & 3,732        & 430         & 0            & 33                & 30               & 23            & 36          & 1         & 141        & 44        & 1,152          & 42              & 26           & 0            \\ \hline
\textbf{Sum}   & \textbf{139,889}      & \textbf{474,716}      & \textbf{623,823}      & \textbf{17,003}        & \textbf{9,987}              & \textbf{781,915}           & \textbf{557,981}        & \textbf{25,999}       & \textbf{1,183,738}   & \textbf{56,754}      & \textbf{81,243}     & \textbf{207,673}        & \textbf{176,740}          & \textbf{1,347,725}      & \textbf{34,934}        \\ \hline
\end{tabular}
}%
\label{tab:01:images-per-label-per-server}
\end{resizebox}
\end{table*}

\begin{table*}[ht]
\centering
\caption{$T=0.3$-second window dataset: Images per class value, per server.}
\begin{resizebox}{\textwidth}{!}{%
\begin{tabular}{|c|c|c|c|c|c|c|c|c|c|c|c|c|c|c|c|c|c|}
\hline
Class & youtube.com & semrush.com & discord.com & instagram.com & mercedes-benz.com & bleacherreport.com & nicelocal.com & facebook.com & pcmag.com & logitech.com & google.com & cdnetworks.com & independent.co.uk & cloudflare.com & jetbrains.com \\ \hline
0 & 11,185 & 23,751 & 26,130 & 2,942 & 1,082 & 107,871 & 19,851 & 1,537 & 316,252 & 3,990 & 7,031 & 8,530 & 31,494 & 45,521 & 3,100 \\ \hline
1 & 12,954 & 56,849 & 22,566 & 1,081 & 214 & 70,024 & 21,724 & 1,510 & 35,476 & 5,041 & 6,702 & 13,318 & 26,392 & 86,815 & 1,713 \\ \hline
2 & 6,569 & 34,403 & 31,911 & 655 & 168 & 37,090 & 23,963 & 640 & 21,239 & 4,459 & 4,465 & 11,463 & 4,968 & 84,493 & 1,622 \\ \hline
3 & 4,651 & 18,272 & 33,139 & 359 & 105 & 18,401 & 23,611 & 917 & 5,272 & 2,663 & 1,954 & 7,993 & 2,075 & 37,014 & 1,005 \\ \hline
4 & 3,447 & 13,116 & 33,214 & 286 & 78 & 11,685 & 18,049 & 768 & 1,427 & 2,261 & 1,617 & 7,114 & 928 & 22,280 & 722 \\ \hline
5 & 6,307 & 12,567 & 23,249 & 143 & 71 & 7,682 & 15,305 & 312 & 768 & 1,629 & 912 & 6,084 & 491 & 14,270 & 732 \\ \hline
6 & 3,745 & 7,098 & 17,279 & 237 & 88 & 6,711 & 12,300 & 167 & 1,077 & 2,182 & 860 & 5,844 & 292 & 13,965 & 741 \\ \hline
7 & 2,918 & 5,823 & 18,919 & 541 & 67 & 8,433 & 9,786 & 2,254 & 1,114 & 739 & 1,293 & 5,140 & 363 & 12,478 & 532 \\ \hline
8 & 1,439 & 4,921 & 13,591 & 238 & 76 & 22,045 & 8,065 & 193 & 1,047 & 511 & 979 & 4,414 & 246 & 10,979 & 1,025 \\ \hline
9 & 815 & 3,624 & 4,322 & 189 & 71 & 12,548 & 7,170 & 63 & 468 & 477 & 529 & 3,350 & 153 & 7,975 & 1,642 \\ \hline
10 & 230 & 3,917 & 2,848 & 190 & 78 & 13,965 & 7,394 & 69 & 358 & 342 & 370 & 2,717 & 117 & 2,784 & 1,505 \\ \hline
11 & 166 & 5,221 & 1,651 & 167 & 62 & 10,530 & 7,527 & 61 & 551 & 335 & 396 & 2,024 & 173 & 954 & 2,383 \\ \hline
12 & 80 & 4,704 & 1,261 & 77 & 50 & 2,464 & 8,338 & 114 & 267 & 360 & 373 & 1,754 & 103 & 641 & 1,677 \\ \hline
13 & 46 & 3,430 & 882 & 7 & 50 & 478 & 9,361 & 185 & 103 & 289 & 317 & 1,336 & 125 & 443 & 71 \\ \hline
14 & 24 & 2,194 & 988 & 0 & 66 & 248 & 10,034 & 713 & 169 & 982 & 274 & 1,055 & 110 & 290 & 0 \\ \hline
15 & 29 & 2,725 & 775 & 0 & 71 & 341 & 7,660 & 293 & 75 & 549 & 273 & 909 & 133 & 152 & 0 \\ \hline
16 & 14 & 3,827 & 669 & 0 & 62 & 232 & 5,217 & 192 & 25 & 444 & 188 & 752 & 58 & 125 & 0 \\ \hline
17 & 10 & 4,288 & 431 & 0 & 60 & 369 & 3,471 & 185 & 33 & 516 & 169 & 626 & 51 & 88 & 0 \\ \hline
18 & 10 & 3,641 & 479 & 0 & 75 & 170 & 2,207 & 356 & 50 & 387 & 152 & 469 & 71 & 93 & 0 \\ \hline
19 & 11 & 3,300 & 408 & 0 & 77 & 104 & 1,177 & 424 & 14 & 262 & 132 & 375 & 78 & 80 & 0 \\ \hline
20 & 9 & 3,806 & 536 & 0 & 69 & 139 & 759 & 35 & 12 & 162 & 82 & 440 & 59 & 48 & 0 \\ \hline
\textbf{Sum} & \textbf{54,659} & \textbf{221,477} & \textbf{235,248} & \textbf{7,112} & \textbf{2,740} & \textbf{331,530} & \textbf{222,969} & \textbf{10,988} & \textbf{385,797} & \textbf{28,580} & \textbf{29,068} & \textbf{85,707} & \textbf{68,480} & \textbf{341,488} & \textbf{18,470} \\ \hline
\end{tabular}
}%
\label{tab:03:images-per-label-per-server}
\end{resizebox}
\end{table*}

%Prior to feeding data into the GRU, we perform a reshaping operation to ensure the GRU layer correctly interprets the time dimension. This transformation preserves the temporal order of the data across 29 time steps. We also experimented with various other time steps during our experiments.
